# Supplementary material for: DEFT: Differentiable Branched Discrete Elastic Rods for Modeling Furcated DLOs in Real-Time
Source: arXiv:2502.15037 source file (2026-10-21)
Supplement: Supplementary file 1 [file appendix_storage.tex]

% \begin{table*}[t]
% \centering
% \caption{A summary of each BDLO's material properties and marker count used in the real-world experiment. Stiffness is estimated based on a relative scale.}
% \label{mat_prop}
% \begin{tabular}{c|| c |c | c| c |c}
% \toprule
% BDLO & \makecell{Parent\\ Stiffness / \#Markers} & \makecell{Child1\\ 
% Stiffness / \#Markers} & \makecell{Child2\\ Stiffness / \#Markers} & \makecell{Dataset 1 \\ Time (s)} & \makecell{Dataset 2 \\ Time (s)} \\
% \hline 

% 1 & Medium / 13 & Medium / 4 & Medium / 3 & 505 & 440 \\
% 2 & Low / 12    & Low / 4    & Low / 4    & 735  & N/A\\
% 3 & Medium / 12 & Low / 2    & High / 3   & 645 & 445\\
% 4 & Medium / 12 & High / 2   & High / 2   & 495 & N/A \\
% \bottomrule
% \end{tabular}
% \end{table*}


% \begin{figure}
%     \centering
%     \includegraphics[width=0.5\textwidth]{figures/experiment_setup.png}
%     \caption{An illustration of experiment setup.
%     Top: Data collection setup with a dual-arm robot. 
%     Bottom: An illustration of the BDLOs used to evaluate and compare the performance of DEFT against baseline methods. 
%     To increase dataset diversity, we vary the BDLOs’ stiffness, length, weights, number of vertices, and junction structures.}    
%     \label{fig:experimentsetup}
% \end{figure}

% % \begin{table}[t]
% % \centering
% % \caption{Modeling Results Over a $5$s Horizon}
% % \begin{tabular}{l||cccc|cc||cccc}
% %     \toprule
% %     & \multicolumn{6}{c||}{Modeling Accuracy (RMSE, $10^{-2}$\,m)} 
% %     &\multicolumn{4}{c}{Time ($10^{-2}$s)}  \\     
% %     & \multicolumn{4}{c|}{Dataset 1} & \multicolumn{2}{c||}{Dataset 2}  & \multicolumn{4}{c}{Dataset 1} \\ 
% %     Method & 1 & 2 & 3 & 4 & 1 & 3 & 1 & 2 & 3 & 4    \\
% %     \hline
% %     GCN \cite{GCN} & 6.70 & 6.42  & 5.25 & 4.20 & 7.33 & 4.24 & \textbf{0.20} & \textbf{0.19} & \textbf{0.13} & \textbf{0.13}\\
% %     Tree-LSTM \cite{treeLSTM} & 5.32 & 4.50 & 2.46 & 2.71 & 7.08 & 4.55 & 1.81 & 2.44 & 1.79 & 1.89\\
% %     FEM: dt: $10^{-6}$s, node: 60 & 3.11 & 3.70 & 2.29 & 2.84 & 2.17 & 2.10 & 487 & 510 &  470  & 504  \\
% %     FEM: dt: $10^{-6}$s, node: 160& 2.07&3.35 & 1.82 & 1.54 & \textbf{1.40} & 1.94 & 1126 & 1290 & 1150 & 1279\\
% %     FEM: dt: $10^{-2}$s, node: 60& 14.6 &18.3 & 12.1 & 17.6 & 14.9 & 12.3 & 0.47 & 0.50 & 0.45 & 0.52  \\
% %     FEM: dt: $10^{-2}$s, node: 160& 12.9 &15.1 & 10.0 & 11.8 & 12.8& 9.71 & 1.16& 1.01 & 0.90 & 1.28\\
% %     DEFORM++ & 4.59 &  7.44 & 5.02 & 4.46 & 3.88 &  4.25 & 1.80 & 1.73 & 1.49 & 1.64  \\
% %     DEFT & \textbf{1.87} &  \textbf{2.82} &  \textbf{1.51} &  \textbf{1.41} & 1.49 &  \textbf{1.80} & 0.76 & 0.70 & 0.91 & 0.93\\
% %     \bottomrule
% % \end{tabular}
% % \label{tab:model accuracy end points1}
% % \end{table}



% \begin{table}[t]
%         \centering
%     \caption{Compuational Time for \eqref{eq:innerloop} with Dataset 1}
%     \begin{tabular}{l||cccc}
%         \toprule
%         & \multicolumn{4}{c}{Time ($10^{-2}$ s)} \\         
%         Method & 1 & 2 & 3 & 4   \\
%         \hline
%         Analytical Gradient & \textbf{0.34} & \textbf{0.27} & \textbf{0.41} & \textbf{0.46}  \\
%         Numerical Gradient & 0.74 & 0.65 & 0.84 & 0.91 \\
%         \bottomrule
%     \end{tabular}
%     \label{tab:computational speed2}
%     \centering
% \end{table}

% \begin{align}
% \label{eq:delta_x}
% \Delta\hat{\mathbf{x}}^a &= \mathbf{M}^b(\mathbf{M}^a + \mathbf{M}^b)^{-1}\,\frac{g(\hat{\mathbf{z}})}{\lVert \mathbf{d}\rVert^2}\,\mathbf{d}, 
% & 
% \Delta\hat{\mathbf{x}}^b &= -\,\mathbf{M}^a(\mathbf{M}^a + \mathbf{M}^b)^{-1}\,\frac{g(\hat{\mathbf{z}})}{\lVert \mathbf{d}\rVert^2}\,\mathbf{d}, \\
% \Delta\hat{\bm{\Omega}}^a &= \mathbf{I}^b(\mathbf{I}^a + \mathbf{I}^b)^{-1}\,\frac{g(\hat{\mathbf{z}})}{\lVert \boldsymbol\delta\rVert^2}\,\boldsymbol\delta, 
% &
% \Delta\hat{\bm{\Omega}}^b &= -\,\mathbf{I}^a(\mathbf{I}^a + \textbf{I}^b)^{}\,\frac{g(\hat{\mathbf{z}})}{\lVert \boldsymbol\delta\rVert^2}\,\boldsymbol\delta,
% \label{eq:delta_omega}
% \end{align}
% where
% $\mathbf{d} = \frac{\partial g}{\partial \hat{\mathbf{x}}^a},
% \boldsymbol\delta = \frac{\partial g}{\partial \hat{\bm{\Omega}}^a}.$
% \label{theorem:constraints}
